# Supplementary material for: $M^3EL$: A Multi-task Multi-topic Dataset for Multi-modal Entity Linking
Source: arXiv:2410.18096 source file (2024-10-08)
Supplement: Supplementary file 1 [file appendix.tex]

\section{The Quality of Candidates for Candidate Filtering}
\label{sec:appendix C}

\begin{figure*}[htbp]
  \begin{subfigure}{1\linewidth}
	\centering
	\begin{subfigure}{\linewidth}
		\centering
		\includegraphics[width=\linewidth]{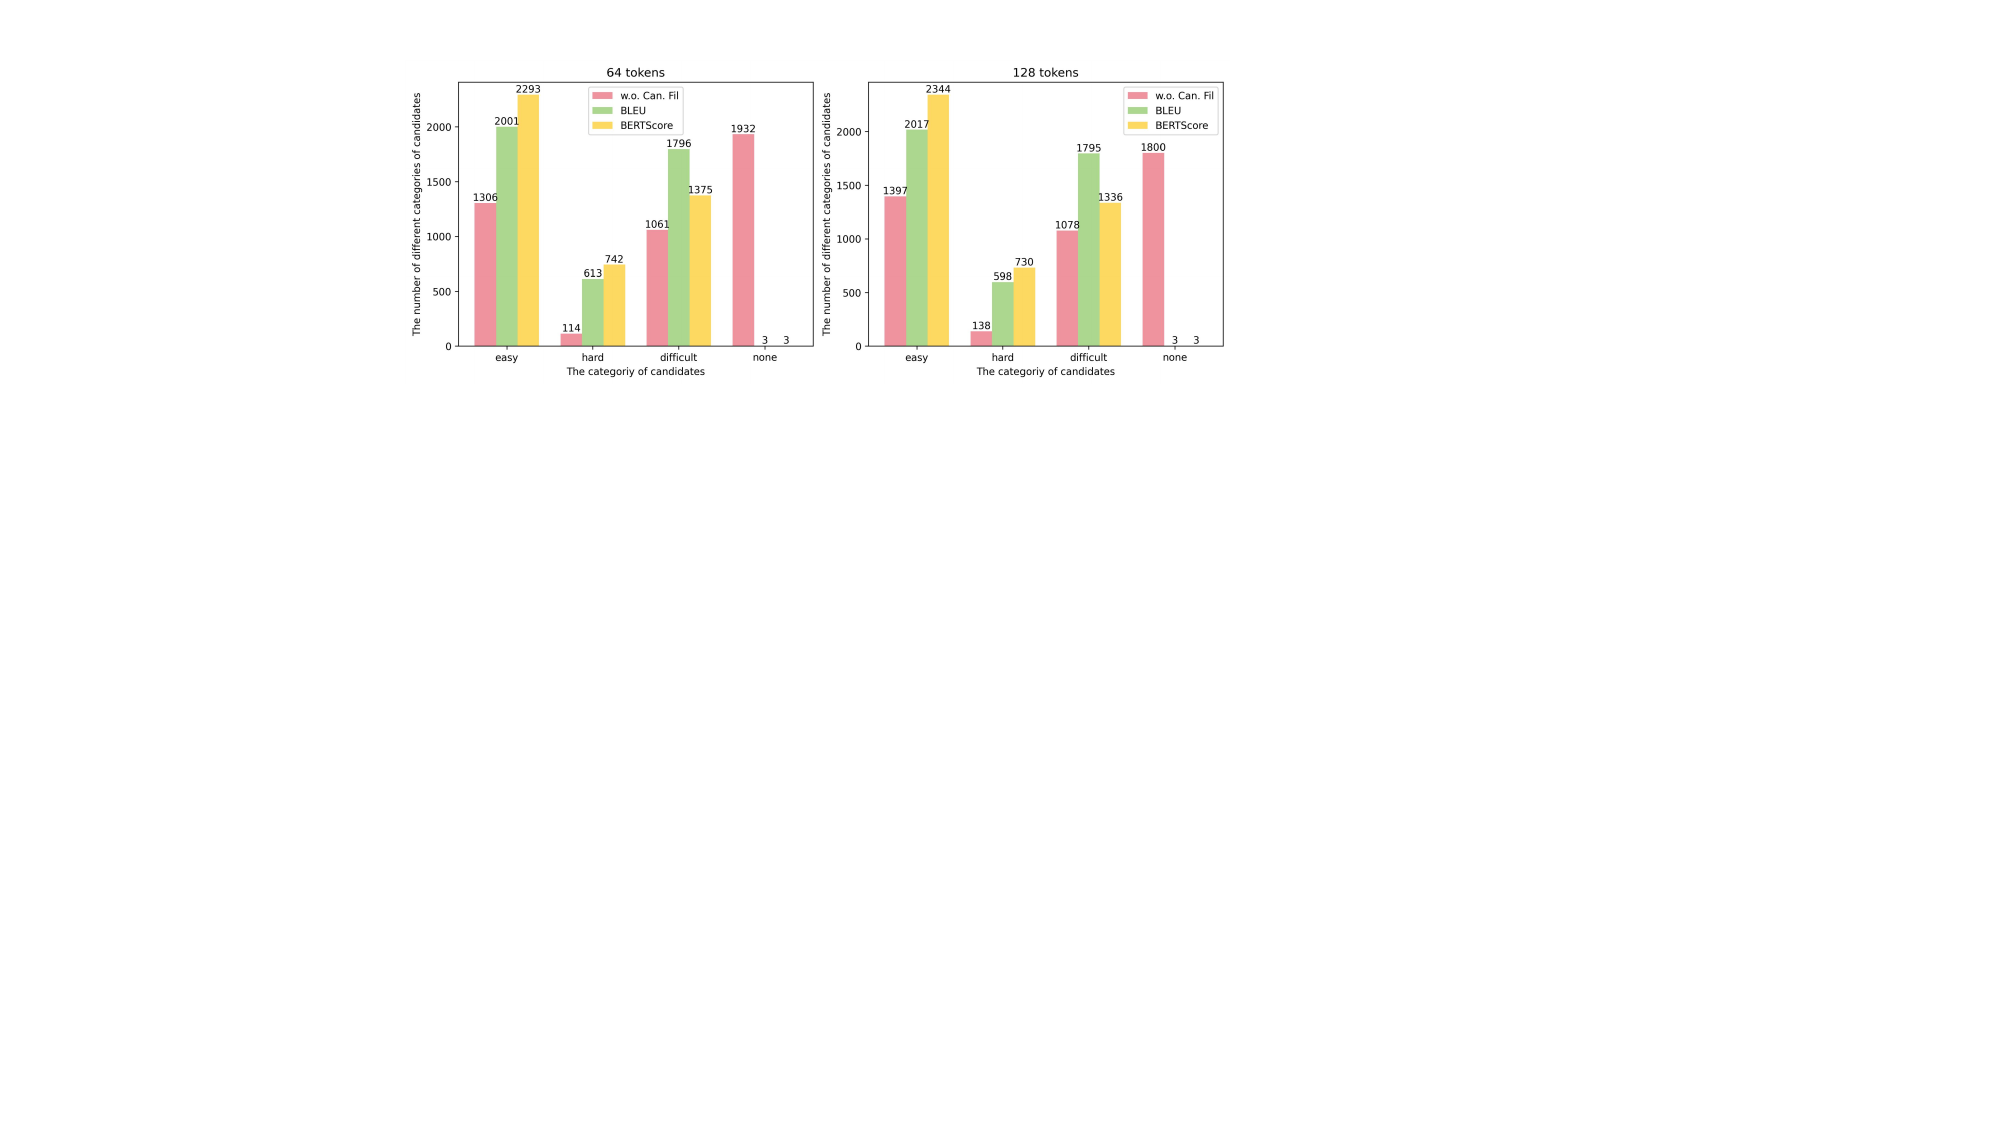}
        \caption{The candidates of Prompt 3-1}
		\label{logical}
	\end{subfigure}
 
	\begin{subfigure}{1\linewidth}
		\centering
		\includegraphics[width=\linewidth]{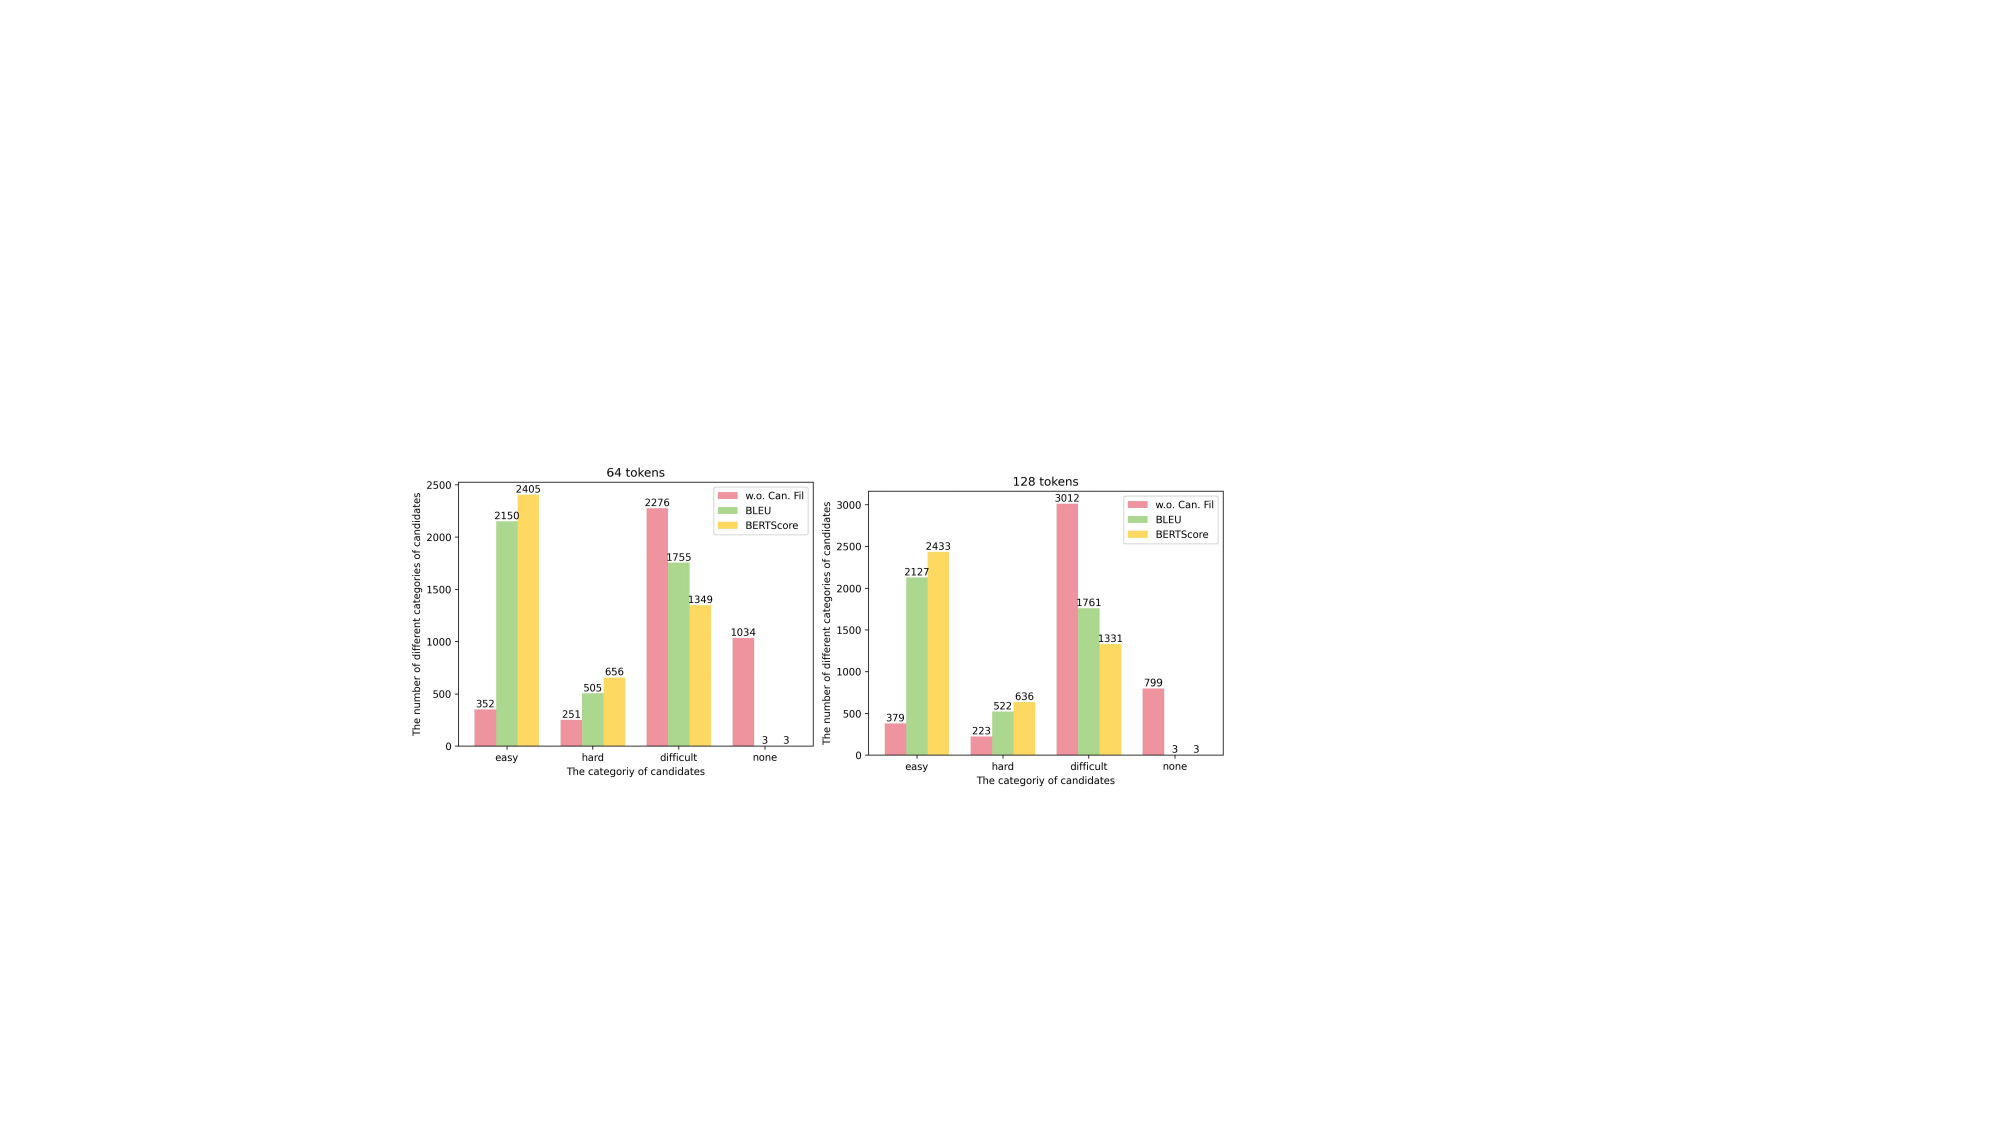}
        \caption{The candidates of Prompt 4-1}
		\label{physical}
	\end{subfigure}
	
  \end{subfigure}
  
\caption{\textbf{Quality Demonstration Graph of Candidates for Candidate Filtering.}} 
\label{fig:p1+p2}
\end{figure*}

\begin{table*}[]
\caption{\textbf{The different examples in semantic understanding prompts.}}
\label{tab:prompt3vs4}
\begin{tabular}{c|l}
\toprule
\textbf{Prompts} & \multicolumn{1}{c}{\textbf{\begin{tabular}[c]{@{}c@{}}Examples of semantic understanding prompt\\ (sentence, description)\end{tabular}}}                                                  \\ \midrule[1pt]
Prompt 3-1       & \begin{tabular}[c]{@{}l@{}}'Soccer-late goals give JAPAN win over SYRIA...',\\  'Japan national football team: national association football team.'\end{tabular}                          \\ \hline
Prompt 4-1       & \begin{tabular}[c]{@{}l@{}}'Soccer-late goals give JAPAN win over SYRIA...', \\ "Japan national football team: men's national association football team representing Japan."\end{tabular} \\
\bottomrule
\end{tabular}
\end{table*}

In our research, both Prompt 3-1 and Prompt 3-0 employ Wikidata to search for the outputs (queries) of semantic understanding prompts. When the initial search yields no results, Prompt 3-1 utilizes a mention as a substitute to conduct a second search. The processing logic for Prompt 4-1 and Prompt 4-0 follows the same methodology. Upon comparison, we found that Prompt 3-1 and Prompt 4-1 respectively outperform Prompt 3-0 and Prompt 4-0 in terms of performance. Thus we compare the quality of candidates between Prompt 3-1 and Prompt 4-1 across various document segmentation by token (64 or 128) in Figure \ref{fig:p1+p2}. Each subfigure presents three distinct scenarios of candidate filtering:

\begin{itemize}
    \item {\textbf{w.o. Can. Fil. : }}Without using Candidate Filtering. Utilizing the term ‘understanding’ returned by semantic understanding prompt as the query, call the dynamic online wikidata to directly search for the query, and obtain the results as the candidates.
    \item {\textbf{BLEU: }}Based on the results of tool invocation and semantic understanding prompt, use BLEU to calculate the similarity of understanding-description pair for filtering candidates.
    \item {\textbf{BERTScore: }}Similar to the step of BLEU.
\end{itemize}

It becomes evident that candidates filtered with BLEU and BERTScore are much better in quality than those without filtering (denoted as w.o. Can. Fil.). Specifically, the number of candidates containing the correct answer (both easy and hard) increases, while the number of candidates without the correct answer (difficult) and those yielding no search results (none) decreases. This is primarily due to the search feature of Wikidata. Wikidata, being a knowledge graph rich in structured knowledge, is adept at searching for entities and their attribute information. Notably, when the target mention aligns closely with the entity name, Wikidata's precision in returning results is higher. However, using queries actually increases the complexity of the Wikidata search. For instance, when searching for ‘\textit{JAPAN}’, Wikidata returns ‘\textit{Japan (Q17)}’ representing the country, and when searching for ‘\textit{The target mention 'JAPAN' refers to a soccer team or national team from Japan, which emerged victorious in a soccer match against Syria.}’, Wikidata returns ‘\textit{There were no results matching the query}’. Therefore, direct search for query from semantic understanding prompt struggle to effectively complete semantic disambiguation and entity linking at once.

Comparing the quality of candidate by BLEU and BERTScore in Prompt 3-1 and Prompt 4-1, it becomes evident that BERTScore outperforms BLEU. This is because BLEU calculates the word repetition of query and description without considering semantic information. However, ChatGPT is a generative model that conveys understanding in the form of natural language, and the pre-trained BERT model can effectively capture semantic information of understanding and descriptions. 

In addition, under the same conditions, the candidate quality of Prompt 4-1 is better than that of Prompt 3-1. This variation is attributed to the different examples of in-context learning provided in each Prompt, which leads to distinct understandings of the mention and influences the similarity scores calculated by BLEU and BERTScore, ultimately affecting candidate quality. 

Table \ref{tab:prompt3vs4} presents an example constituted by a \textbf{tuple (sentence, description)}, where the \textbf{sentence}, indicating the context of the mention, remains consistent between Prompt 3-1 and Prompt 4-1. However, the \textbf{description} in Prompt 3-1 is derived from the original dataset's explanation of the mention, while the \textbf{description} in Prompt 4-1 comes from Wikidata's description of the mention. Given that descriptions from Wikidata are more current and accurate, the original dataset's explanations may contain errors due to their temporal limitations. Consequently, the candidate quality in Prompt 4-1 is superior to that in Prompt 3-1, further underscoring the necessity of utilizing online dynamic Wikidata as a replacement for the original static dataset (knowledge graph).

\section{Different $Sea\_can$ \& $Sim\_can$}
\label{sec:appendix D}

In Table ~\ref{tab: Different combinations of cans}, we present different combinations of $Sea\_can$ and $Sim\_can$ used to construct the candidate sets $Cans$.

\begin{itemize}
    \item $Sea\_can$ refers to candidates that are constructed from the top-5 results obtained through searching mention on Wikidata.
    \item $Sim\_can$ refers to candidates that are constructed from the top-5 results obtained through BERTScore(query, description).
    \item $Sea\_can + Sim\_can$ refers to the candidates from $Sim\_can$ are appended to those in $Sea\_can$.
    \item $Sim\_can + Sea\_can$ refers to the candidates from $Sea\_can$ are appended to those in $Sim\_can$.
\end{itemize}

The precision of $Sea\_can$ surpasses that of $Sim\_can$. This superiority is attributable to Wikidata's robust search and matching capabilities, which yield higher quality results for mention searches. Additionally, when employing the BERTScore model, the model exhibits varying preferences for different vocabularies. Relying solely on the obtained candidates can inadvertently lower the correct candidate's rank among the candidates. Based on these observations, we conducted experiments involving the combination of two subsets of candidates.

\begin{table}[]
\caption{\textbf{Different combinations of $Sea\_can$ and $Sim\_can$  to construct the $Cans$ in AIDA-B dataset.}}
\label{tab: Different combinations of cans}
\centering
\setlength{\tabcolsep}{4mm}{\begin{tabular}{ccccc}
\toprule
    \multirow{2}{*}{\textbf{Combines}}& \multicolumn{2}{c}{\textbf{64 tokens}} & \multicolumn{2}{c}{\textbf{128 tokens}} \\
          \cmidrule(lr){2-3} \cmidrule(lr){4-5}
    &Sen & Men & Sen & Men  \\ \hline
    $Sea\_can$               &0.65  & 0.66  & 0.67  & 0.68 \\
    $Sim\_can$               &0.47  & 0.49  & 0.51  & 0.54 \\ \hdashline
    $Sim\_can$ + $Sea\_can$  &0.56  & 0.59  & 0.61  & 0.64 \\
    $Sea\_can$ + $Sim\_can$  &0.69  & 0.71  & 0.70  & 0.78 \\
\bottomrule
\end{tabular}}
\end{table}

The precision of $Sea\_can + Sim\_can$ surpasses that of $Sim\_can + Sea\_can$, primarily due to the search results from Wikidata appearing in the upper half of the candidate list. The LLMs exhibit a deeper memory for information encountered earlier, which in turn enhances the quality of multi-choice, thereby increasing the precision of entity linking.

\begin{table}[]
\caption{\textbf{Effect of the different question of multiple choice prompt.} The can\_X indicates the number of candidates is X.}
\label{tab: different questions}
\centering
\setlength{\tabcolsep}{3mm}{\begin{tabular}{cccc}
\toprule
    \textbf{Questions} &\textbf{Can\_5} &\textbf{Can\_10} &\textbf{Can\_20} \\ \hline
    sentence  &0.711   &0.774  &0.752  \\
    summary   &0.713   &0.774  &0.760\\
    understanding   &0.718   &0.783   &0.764\\
\bottomrule
\end{tabular}}
\end{table}

\begin{table}[!b]
\caption{\textbf{The analysis of static offline knowledge graph lacks time-sensitive.} The "-X\%" denotes the random removal of X\% of data from the raw dataset.}
\label{tab:ablation for MC}
\centering
\small
\begin{tabular}{ccccc}
\toprule
    \textbf{Mentions} &\textbf{AIDA} &\textbf{WNED-Wiki} & \textbf{WNED-Cweb} & \textbf{Wiki-Wiki}  \\ \midrule[1pt]
    -70\%  &0.18  &0.14  &0.18  &0.27   \\
    -50\%  &0.35  &0.23  &0.26  &0.41   \\
    -30\%  &0.45  &0.30  &0.34  &0.52   \\ 
    -10\%  &0.56  &0.35  &0.36  &0.64   \\ \midrule[0.5pt] 
    all    &0.64  &0.47  &0.48  &0.76   \\
\bottomrule
\end{tabular}
\end{table}

\section{Different question of multiple choice}
\label{sec:appendix E}

In Table ~\ref{tab: different questions}, "sentence" denotes the sentence with the mention, "summary" comes from SumMC, and "understanding" is from OUEL.

The results indicate that when employing the three terms as the question of multiple choice prompts for entity linking, the precision achieved by each prompt does not differ much. Notably, the precision of the understanding is marginally higher, attributable to the detailed steps incorporated within the semantic understanding prompt. These steps effectively exploit the LLM comprehension capability.

The number of candidates affects multiple-choice  results, with 10 candidates giving the best results. Having too few candidates (can\_5) means the correct option might not be covered. In contrast, having too many (can\_20) makes the text too long and complicates the selection process for LLMs due to their varied memory for differently sequenced information.

\section{Timeliness of static knowledge graph}
\label{sec:appendix F}

In Table ~\ref{tab:ablation for MC}, we initiate an analysis of the impact of static offline knowledge graphs on the performance of the baseline SumMC. Specifically, we conducted experiments in which we randomly removed 10\%, 30\%, 50\%, and 70\% of mentions from the original dataset, simulating a scenario in which static offline knowledge graphs lack updates for mentions in the real world. 

The experimental results reveal that when a substantial number of unknown target mentions are present, the effectiveness of SumMC experiences a significant decline. For example, in the case of the Wiki-Wiki dataset, the removal of 70\% of target mentions results in a reduction of precision from 76\% to 27\%. Consequently, the invocation of tools, specifically the substitution of a static offline knowledge graph with a dynamic online KG, becomes highly necessary and meaningful.

% \section{Details of Prompts}
% \label{sec:appendix G}

% The details of multiple choice prompt and semantic understanding prompt are shown in Figures ~\ref{fig:Multiple-Choice-prompt} and ~\ref{fig:semantic-understanding-prompt}, respectively.

% \begin{figure*}[htbp]
% \centering
% \includegraphics[width=\textwidth]{figures/MCP.pdf} 
% \caption{\textbf{Prompt for multiple choice.}}
% \label{fig:Multiple-Choice-prompt}
% \end{figure*}

% \begin{figure*}[htbp]
% \centering
% \includegraphics[width=0.85\textwidth]{figures/SUP.pdf} 
% \caption{\textbf{Prompt for semantic understanding.} The different examples are show in various prompts.}
% \label{fig:semantic-understanding-prompt}
% \end{figure*}
