# Supplementary material for: $M^3EL$: A Multi-task Multi-topic Dataset for Multi-modal Entity Linking
Source: arXiv:2410.18096 source file (2024-10-08)
Supplement: Supplementary file 2 [file prompt_appendix.tex]

\section{Details of Prompts}
\label{sec:appendix A}

The details of multiple choice prompt and semantic understanding prompt are shown in Figures ~\ref{fig:Multiple-Choice-prompt} and ~\ref{fig:semantic-understanding-prompt}, respectively.

\begin{figure}[b]
\centering
\includegraphics[width=0.5\textwidth]{figures/MCP.pdf} 
\caption{\textbf{Prompt for multiple choice.}}
\label{fig:Multiple-Choice-prompt}
\end{figure}

\begin{figure}[b]
\centering
\includegraphics[width=0.5\textwidth]{figures/SUP.pdf} 
\caption{\textbf{Prompt for semantic understanding.} The different examples are show in various prompts.}
\label{fig:semantic-understanding-prompt}
\end{figure}
